# Supplementary material for: Virtual Guidance as a Mid-level Representation for Navigation with Augmented Reality
Source: arXiv:2303.02731 source file (2025-03-14)
Supplement: Supplementary file 1 [file 5_appendix.tex]

\subsubsection{Static and Dynamic Obstacles}
The virtual environments in our simulation incorporate both static and dynamic obstacles to emulate real-world navigation challenges. Static obstacles are introduced as randomly placed obstacle boxes on the ground along the route. On the other hand, simulated road-crossing pedestrians, which serve as dynamic obstacles, are instantiated at various points in the environment with an initial random speed $V_{walk}$ and a random acceleration $a_{walk}$. These pedestrian agents are configured to cross the road from either the left or the right side. The emergence of pedestrian agents in the simulation is governed by a duration calculated as $1 / (D_{ped} \times \hat{V}_{walk})$ seconds, where $D_{ped}$ denotes the predefined pedestrian density in the environment, and $\hat{V}_{walk}$ represents the average walking speed of the pedestrians. This spawn rate is adjusted to maintain a steady flow of pedestrians and is designed to ensure the alignment with the traffic load conditioned by $D_{ped}$. When reaching their predetermined destination on the opposite side of the pathway, the pedestrians are removed from the simulation. 

\subsubsection{An Overview of the Real-World Framework}
Fig.~\ref{fig:overview} illustrates an overview of our framework for real-world evaluation. To validate the applicability of the proposed virtual guidance scheme in practical scenarios, we have designed real-world tasks with two objectives. First, these tasks should verify the effective transferability of the pre-trained DRL agent's policy to real-world settings, where it follows the virtual guidance. Second, they should demonstrate that the virtual guidance scheme possesses the flexibility to adapt not only to trajectories generated by specific planning algorithms but also to instructions from different methods, such as text prompts or natural language descriptions. This real-world setting aims to validate that the virtual guidance scheme possesses adaptability, and allows guidance generation from other sources or modalities as long as such signals can be translated into visual representations.
